# Supplementary material for: Laser-generated GHz surface acoustic waves with tunable amplitude during the magnetostructural phase transition in FeRh thin films
Source: arXiv:2511.09318 ancillary file (2026-02-18)
Supplement: Supplementary file 1 [file SUPPLEMENT.pdf]

# Supplemental Material: Tunable laser-generated GHz surface acoustic waves during magnetostructural phase transition in FeRh thin films

Ia. A. Mogunov,<sup>1,\*</sup> A. Yu. Klovov,<sup>2</sup> N. Yu. Frolov,<sup>2</sup> A. V. Protasov,<sup>3</sup> G. E. Zhezlyayev,<sup>3</sup>  
D. I. Devyaterikov,<sup>3</sup> R. R. Gimaev,<sup>4</sup> V. I. Zverev,<sup>5</sup> and A. M. Kalashnikova<sup>1</sup>

<sup>1</sup>*Ioffe Institute, 194021 St. Petersburg, Russia*

<sup>2</sup>*P.N. Lebedev Physical Institute of the RAS, 119991 Moscow, Russia*

<sup>3</sup>*Institute of Metal Physics of the Ural Branch of the RAS, 620108 Ekaterinburg, Russia*

<sup>4</sup>*Faculty of Mechanical Engineering,*

*University of Ljubljana, 1000 Ljubljana, Slovenia*

<sup>5</sup>*Lomonosov Moscow State University, 119991 Moscow, Russia*

(Dated: November 6, 2025)

## I. CHARACTERIZATION OF THE SAMPLE

### A. X-ray investigation of FeRh growth

XRD and XRR measurements were performed on PANalytical Empyrean diffractometer in parallel beam geometry using Cu  $K\alpha_1$  radiation. Our sample is a  $\text{Fe}_{49}\text{Rh}_{51}$  film on a single-crystalline (001) MgO substrate with Au capping layer grown by molecular beam epitaxy (for details of growth see [1]). FeRh has cubic CsCl-type crystal structure [2] which is tetragonally distorted due to lattice mismatch with the substrate [3–6]. Thicknesses of the layers and roughness of interlayer boundaries are estimated by fitting X-ray reflectivity (XRR) curve (Fig. 1S(a)). For FeRh layer thickness of 60 nm was obtained with roughness of both layer boundaries less than 0.3 nm, while Au layer was found to be 2 nm and roughness of its boundary with air is 0.7 nm.

X-ray diffraction (XRD) pattern (Fig. 1S(b)), measured in symmetrical geometry provides orientational relation between FeRh layer and MgO substrate in the out-of-plane direction: (001) FeRh|| (001) MgO. Apparently, capping layer has also grown epitaxially, which is evident by the presence of (002) Au and (004) Au reflections on XRD pattern. Width and magnitude of these reflections confirm the small thickness of Au layer.

It is known [3], that in the in-plane direction FeRh lattice is rotated by  $45^\circ$  with respect to MgO lattice. This was confirmed for the studied sample by XRD measurements of (112) and (202) FeRh reflections and (113) MgO reflection in asymmetrical geometry (Fig. 1S(c)). The absence of FeRh grains with different in-plane orientation was further elaborated with 2D scan through  $\phi$  and  $\omega$  axes in asymmetric geometry, where only four reflections corresponding to in-plane orientational relation (100) FeRh|| (110) MgO are present (Fig. 1S(d)). This points toward conclusion that the film was grown single-crystalline as in several other works [7, 8]. Interplanar spacings obtained from (202) and (002) FeRh reflections allowed to determine FeRh lattice parameters at room temperature: in-plane  $a=2.980$  Å, out-of-plane  $c=2.992$  Å, indicating slight tetragonal distortion attributed to epitaxial strain. The resulting epitaxial strains are -0.37 % for  $a$  and 0.03 % for  $c$  considering bulk  $\text{Fe}_{49}\text{Rh}_{51}$  lattice constant at room temperature  $a_{\text{bulk}}=2.991$  Å[9]. The values of  $a$  and  $c$  are in line with previously reported for thin epitaxial FeRh films on (001) MgO [3–6, 10, 11].

---

\* mogunov@mail.ioffe.ru

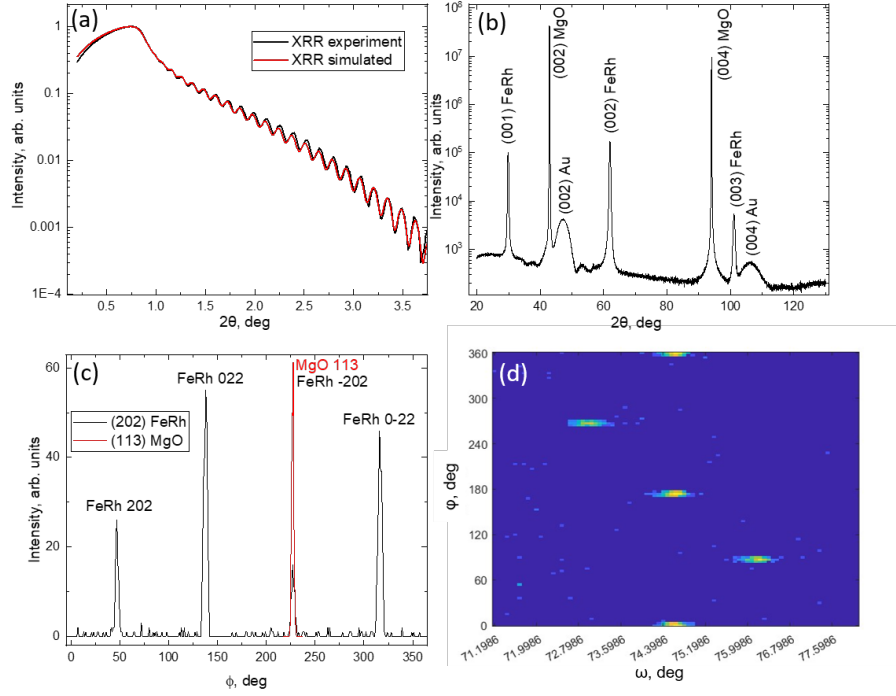

FIG. 1S. **X-ray characterisation of the used sample.** (a) Experimental and fitted X-ray reflectivity (XRR) curve, (b) XRD  $\theta-2\theta$  scan, (c) XRD  $\phi$ -scans in asymmetrical geometry through (113) MgO and (202) FeRh reflections, (d) 2D XRD  $\omega-\phi$  scan of (112) FeRh reflections in asymmetrical geometry.

## B. Atomic force microscopy

Atomic force microscopy was performed at room temperature in semi-contact topology mode using a NT-MDT NTEGRA atomic force microscope with non-magnetic cantilevers. The image (Fig. 2S) shows the sample surface which is a gold protective layer. The root mean square roughness is  $<1.2$  nm which is close to the XRR measurement results. Some irregularities can be seen, their lateral size is smaller than that of the laser spot ( $0.7 \mu\text{m}$ ).

It is known that parameters of AFM-FM phase transition in FeRh alloy are very sensitive to its composition, impurities and defects [10, 12] which depend on the post-growth treatment [7, 9, 13]. In our considerations this would be seen as an additional source of PIPT-threshold distribution on the FM nucleation sites, see Sec. V. We note that the influence of local nonstoichiometry and defects are already included in measured film parameters, namely its thermal hysteresis (Fig. 1(b) of the main text) and determined  $W_T$  and  $W_S$  (inset

on Fig. 1(d) of the main text).

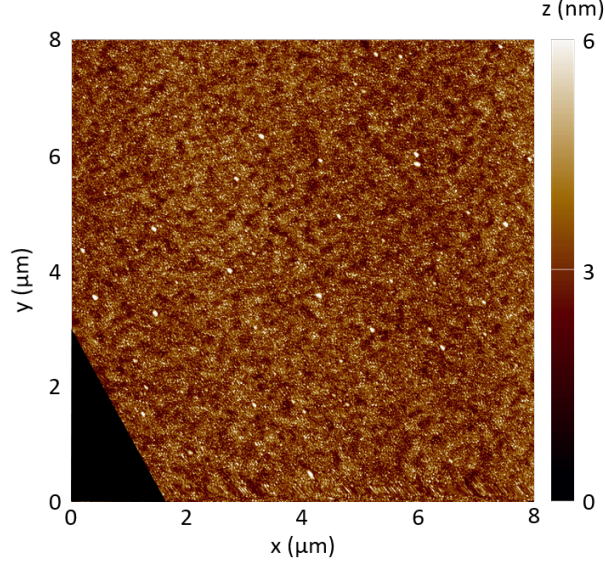

FIG. 2S. Atomic force microscopy image of the sample.

### C. Magnetization measurements

Magnetization measurements were performed using Lake Shore vibration sample magnetometer. Magnetic field was applied in sample plane along  $[110]_{\text{FeRh}}$  direction. We measured  $M(T)$  and  $M(H)$  curves to characterize the AFM-FM phase transition in our sample. Figure 3S shows  $M(H)$  curves measured at several initial sample temperatures  $T_0=300$  K (blue), 330 K (green) and 430 K (red). One can see a small magnetization present at low temperatures when the FeRh film is nominally in AFM phase with coercive field  $\mu_0 H=25$  mT. This means that some FM regions persist down to 300 K which is expected for materials with 1st order phase transitions and specifically for FeRh [14]. The FM phase fraction at 300 K is larger for thinner films [15]. From  $M_{300K}^{\text{max}}/M_{430K}^{\text{max}}$  we estimate the remanent FM phase fraction at 300 K to be 6 %. At  $T_0=430$  K FeRh film is in FM phase, the coercive field is  $\mu_0 H=6$  mT.

The values of  $\mu_0 H$  above which the 'up' and 'down' branches of hysteresis coincide are marked with vertical lines on Fig 3S. These values are closer to zero than  $\mu_0 H=100$  mT chosen for  $M(T)$  measurement (marked with dashed vertical line). The dependencies  $M(H)$  (Fig. 3S) and  $M(T)$  (Fig. 1(b) of the main text) complement each other.

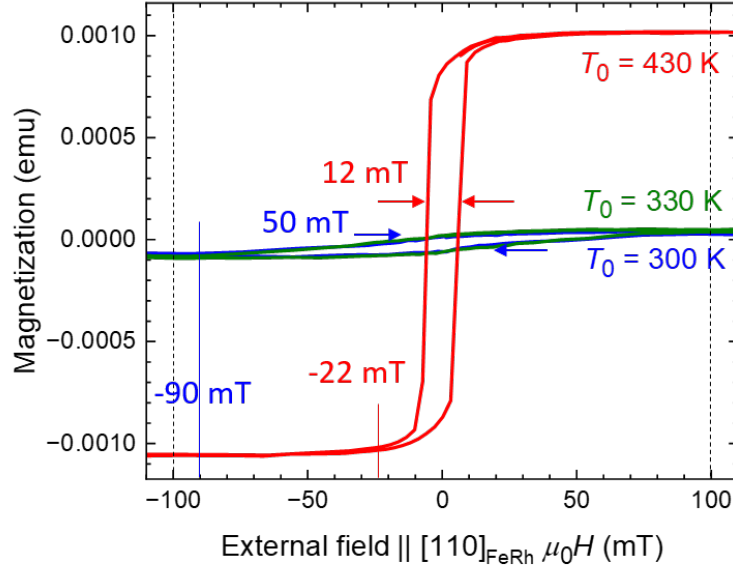

FIG. 3S. **Magnetization vs external magnetic field hysteresis.** The hystereses were measured for three initial sample temperatures: 300 K (blue), 330 K (green) and 430 K (red). Widths of hystereses (equal to double the coercive field) are shown with double arrows. The fields at which there is no further difference between up and down branches are marked with vertical lines.

## II. EXPERIMENTAL PUMP-PROBE SETUPS WITH PHOTOELASTIC SAW DETECTION

The optical scheme is presented on Fig. 4S. We used an Yb:KGW optical system consisting of a femtosecond oscillator TEMA (Avesta Project) in tandem with optical parametric oscillator TOPOL (Avesta Project) working at 70.6 MHz repetition rate with 150 fs pulse duration. Linearly polarized pump pulses with wavelength 680 nm were modulated by an acousto-optical modulator at 997 kHz frequency and were focused by  $\times 50$  micro-objective (numerical aperture 0.5) on the sample surface with normal incidence. Circularly polarized probe pulses with wavelength 525 nm traveled via a mechanical delay line, were directed on a piezoelectric mirror, steered through the  $4f$  system and focused by the same micro-objective. Pump penetration depth in AFM and FM FeRh is 20 nm and 37 nm, correspondingly [8]. Probe penetration depth in AFM and FM FeRh is 24 nm and 29 nm, correspondingly [8]. We optimized focusing of pump and probe simultaneously using telescopes and controlled

the focusing by a digital camera looking at the sample via reflected probe pathway. We put our micro-objective on piezoelectric 3-axis translation stage for precision control of the beam focusing. Pump and probe spots on the sample surface were circular, their FWHM =  $0.9\ \mu\text{m}$  and  $0.7\ \mu\text{m}$ , respectively, as defined by knife-edge method. We measured laser spot sizes on the sample using our FeRh film as an edge and monitoring the intensity of reflected probe or pump light, the scanning across the edge was performed by shifting the micro-objective with piezo translation stage.

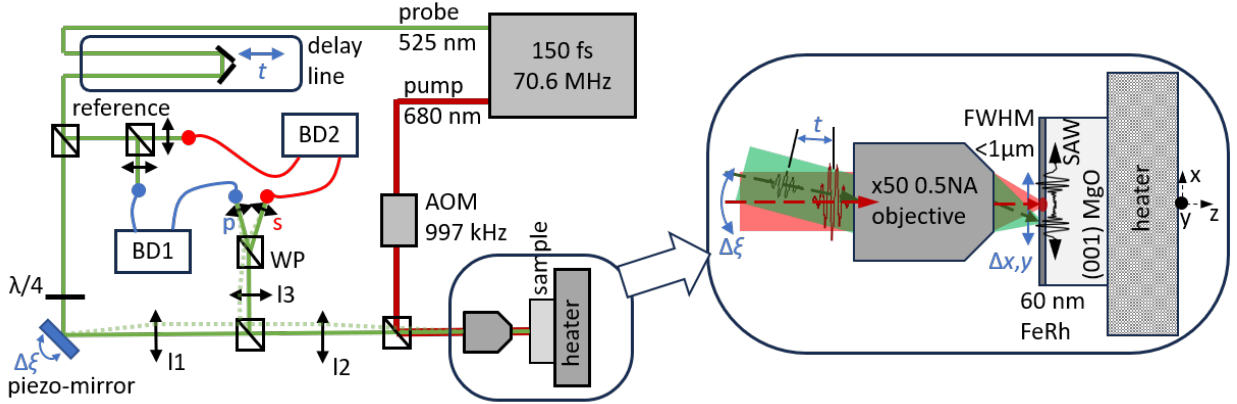

FIG. 4S. **Optical scheme of experimental pump-probe microscopy setup with photoelastic detection of SAWs.** AOM - acousto-optical modulator,  $\lambda/4$  - quarter wave-plate, BD1, BD2 - balanced detectors, WP - Wollstone polarizing prism, lenses  $l1$ - $l2$  and  $l2$ - $l3$  form two  $4f$  systems. Dotted line shows beam path declined by piezoelectric mirror by angle  $\Delta\xi$ ; The inset shows a close-up on the sample, illustrating scanning procedure.  $\Delta\xi$  angle-of-incidence change translates to  $\Delta x$  or  $\Delta y$  shift of probe laser spot on the sample surface.

In experiments we detected intensity of probe pulses reflected from the sample, monitoring separately their  $p$ - and  $s$ - polarization components. This approach allows access to various strain and photoelastic tensor elements and was first implemented by Saito et al. [16]. We use balanced detection with a reference beam to enhance signal-to-noise ratio. In experiments we used lock-in detection on pump modulation frequency for both  $s$ - and  $p$ - components of reflected probe beam and we measure separately their total reflectivities  $R_s$  and  $R_p$ . To do it we used two balanced detectors and for each collected the enhanced balanced signal as well as direct monitor output. Time resolution defined by a mechanical delay line was  $<100$  fs while spatial resolution defined by the piezoelectric mirror and optical scheme was

0.3  $\mu\text{m}$ . The sample is mounted on a resistive heater allowing temperature control with 1 K precision for up to 500 K. We allowed the temperature to stabilize for at least an hour after changing the sample temperature and compensated for the sample shift due to heating by shifting the micro-objective.

### III. SAW VELOCITY EVALUATION

To evaluate the velocities of the studied SAW pulses we used the main setup used in the paper (see Fig. 4S) and performed line scans along  $x$  direction for several time delays  $t=3$ , 5 and 7 ns. The results are shown on Fig. 5S(a).

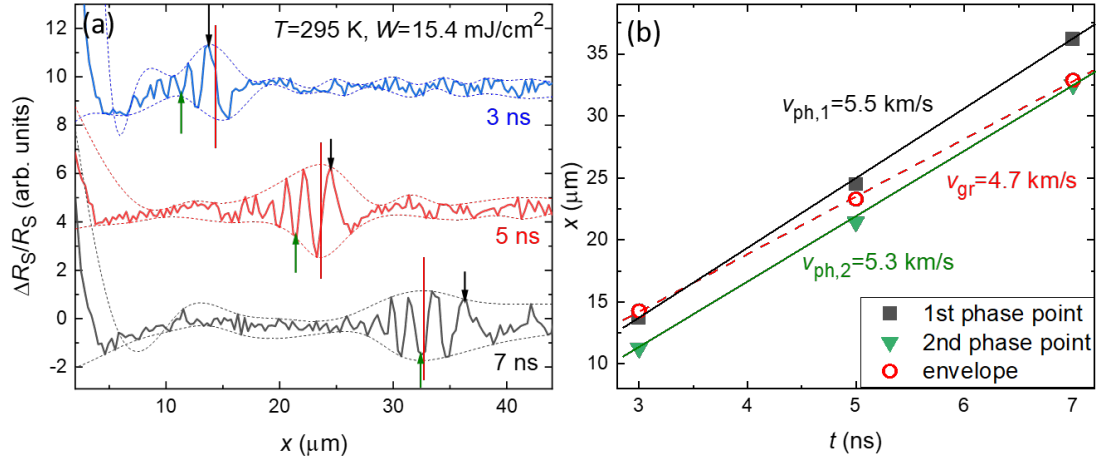

FIG. 5S. **Evaluation of the detected SAW phase and group velocities.** The measurements were performed at  $T=295$  K and pump fluence  $W=15.4$  mJ/cm<sup>2</sup>. (a) Measured  $x$  scans of  $\Delta R_S/R_S$  at several delays  $t=3$  ns (blue), 5 ns (red) and 7 ns (black). Dashed lines show corresponding envelopes. Black and green vertical arrows pinpoint the same-phase parts of the SAW pulse, red vertical line show the maximum of envelope; (b) The  $x(t)$  dependencies of the two same-phase parts of the SAW pulse (black squares and green triangles) and the maximum of envelope (red open circles). The evaluated acoustic velocities are shown with corresponding colors.

We followed the points of the same phase (maxima and minima) of the SAW signal shape and plotted their positions for each of the time delays. The examples for the two same-phase parts marked with arrows on Fig. 5S(a) are shown on Fig. 5S(b). We found that the phase

velocity  $v_{ph}$  diminishes for tail parts of the SAW pulse which is due to acoustic dispersion [17] and the highest value is  $v_{ph,1}=5.5$  km/s. The group velocity was evaluated by constructing envelope functions (dotted lines on Fig/ 5S(a)). Their positions vs time delay are shown with red open circles on Fig. 5S(b) and one can readily see that the group velocity is lower than the phase one. This indicates normal dispersion expected for the lowest SAW quasi-Rayleigh branch in a case when a film loads a substrate [18]. We found the value of  $v_{gr}=4.7$  km/s. It should also be noted that the group velocity depends on the acoustic frequency [17], which in our case is 3.1 GHz.

#### IV. ESTIMATION OF $\varepsilon_{PT}^{SAW}$

Here we clarify an estimation of PIPT-induced contribution to the SAW generation,  $\varepsilon_{PT}^{SAW}$ , recalculating it from the total laser-induced lattice change  $\varepsilon_{PT}$ . The estimation was performed in two steps. On the first step we estimated time-dependence and value of phase-transition-induced pressure  $P(t)$ .

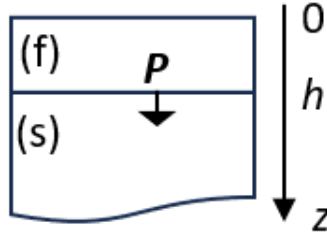

FIG. 6S. **Scheme of the considered system.** (f) is a film with thickness  $h$ , (s) is an infinite substrate. Pressure  $P$  is directed along normal  $z$  and acts on the film/substrate interface.

To do it we considered a film (f) on a substrate (s), the axis  $z$  is directed into substrate,  $z=0$  is free surface,  $z=h$  is film-substrate interface (see Fig. 6S). We only considered strain along  $z$  direction. The equations of motion are:

$$\begin{aligned} -\omega^2 u_z^{(f)} &= v_{(f)}^2 \frac{\partial^2 u_z^{(f)}}{\partial z^2} \\ -\omega^2 u_z^{(s)} &= v_{(s)}^2 \frac{\partial^2 u_z^{(s)}}{\partial z^2}, \end{aligned} \tag{1}$$

where  $u_z^{(f),(s)}$  is displacement of material points and  $v_{(f),(s)}$  – longitudinal elastic wave velocity in film and substrate, correspondingly. The time dependence  $\exp(-i\omega t)$  is omitted.

The boundary conditions are:

$$\begin{aligned}\sigma_{zz}^{(f)}|_{z=0} &= -K^{(f)}(\delta h/h)H(t) + \rho_{(f)}v_{(f)}^2 \frac{\partial u_z^{(f)}}{\partial z}|_{z=0} = 0 \\ \sigma_{zz}^{(f)}|_{z=h} &= -K^{(f)}(\delta h/h)H(t) + \rho_{(f)}v_{(f)}^2 \frac{\partial u_z^{(f)}}{\partial z}|_{z=0} = \rho_{(s)}v_{(s)}^2 \frac{\partial u_z^{(s)}}{\partial z}|_{z=0} = \sigma_{zz}^{(s)}|_{z=0} \\ u_z^{(f)}|_{z=h} &= u_z^{(s)}|_{z=0},\end{aligned}\tag{2}$$

where  $K$  is bulk modulus,  $\rho$  – mass density,  $(\delta h/h)$  is thickness change due to AFM-FM phase transition equal to  $6 \times 10^{-3}$  which is a measured lattice change in  $z$  direction [15] considered by the model.  $H(t)$  is a normalized function containing time-dependence of the film expansion. The first line in Eq. (2) corresponds to a free surface while second and third lines describe continuity of stress and displacement on the film/substrate boundary.

Solving system Eq. (1) with boundary conditions Eq. (2) we find impulsive stress (pressure) originating from the film during phase transition and acting on the substrate surface:

$$P(\omega) = \sigma_{zz}^{(f)}|_{z=h} = K^{(f)}(\delta h/h)H(\omega) \frac{Z_{(s)}[1 - \cos(\omega h/v_{(f)})]}{Z_{(s)} \cos(\omega h/v_{(f)}) - iZ_{(f)} \sin(\omega h/v_{(f)})},\tag{3}$$

where  $Z = \rho v$  is acoustic impedance.

The used temporal dependence of film expansion during phase transition  $H(t)$  is shown on Fig. 7S(a). The time dependence of pressure was found via complex Fourier series:

$$P(t) = \sum_{n=-N}^N P(\omega_n) a_n \exp(-i\omega_n t),\tag{4}$$

where  $\omega_n = \frac{2\pi}{\tau}n$ .  $a_n$  are Fourier amplitudes in  $H(\omega)$  while  $\tau$  is the time period of the Fourier expansion.

The summation was performed by fast Fourier transform. The calculated pressure  $P$  on the substrate surface is shown on Fig. 7S(b). We used MgO substrate parameters: longitudinal and transverse sound velocities  $v_L=9614$  m/s,  $v_T=5949$  m/s,  $\rho=6100$  kg/m<sup>3</sup>. For FeRh we used parameters of laser-induced expanding FM phase:  $v_L=4900$  m/s,  $v_T=2800$  m/s,  $\rho=9580$  kg/m<sup>3</sup> [19].

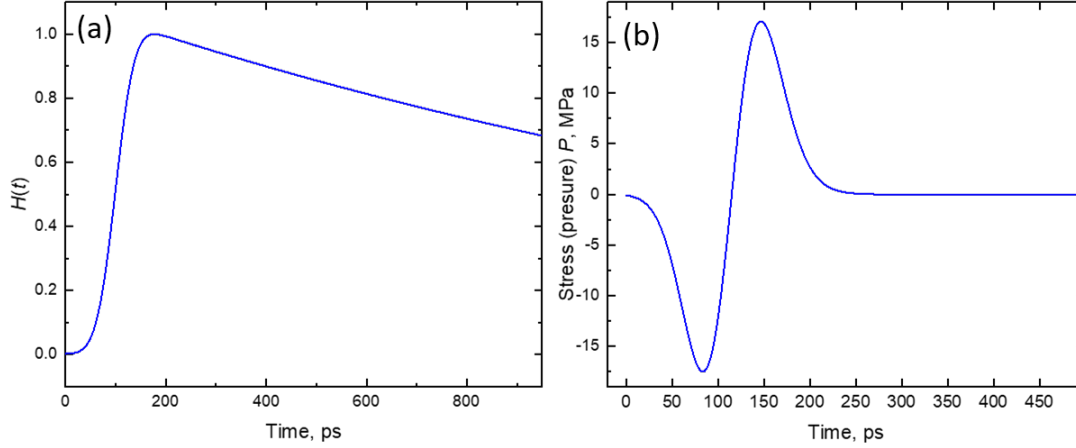

FIG. 7S. **Calculation of pressure due to phase transition in FeRh.** (a) The modeled simplified time evolution of lattice change,  $H(t)$ ; (b) The resulting estimation for FeRh film pressure on the MgO substrate surface,  $P$ .

On the second step of our calculations we used the obtained  $P(t)$  to evaluate the generated SAW amplitude. We utilized the problem for Rayleigh SAW generation in an isotropic half-space by a grating considered in works [20, 21] and put the number of grating periods to one effectively generating SAW by a single stripe with optimized width  $0.34 \mu\text{m}$ . Thus we model the region where AFM-FM transition occurs in a 2D problem: in-plane direction is  $x$  while out-of-plane is  $z$ . The pressure is applied only along  $z$  and is distributed equally under any point of the stripe. The result of calculations is a time evolution of presented on Fig. 8S.

We calculate the strain profile far away from the point of excitation. The time delay on Fig. 8S is set to 5.65 ns to ensure no bulk waves are adding to the shape because in this model bulk waves attenuate while SAWs have no attenuation. The estimated SAW strain components induced by the AFM-FM phase transition are  $\varepsilon_{PT,xx}^{SAW} = 4 \times 10^{-5}$  and  $\varepsilon_{PT,zz}^{SAW} = 1 \times 10^{-5}$  for the used initial phase transition strain  $6 \times 10^{-3}$ . This allows us to estimate the value of a coefficient between SAW in-plane strain and laser-generated strain:  $s = \varepsilon_{xx}^{SAW} / \varepsilon = 4 \times 10^{-5} / 6 \times 10^{-3} = 0.067$ . We note that in this estimation the relation between in-plane and out-of-plane strain components is defined by MgO.

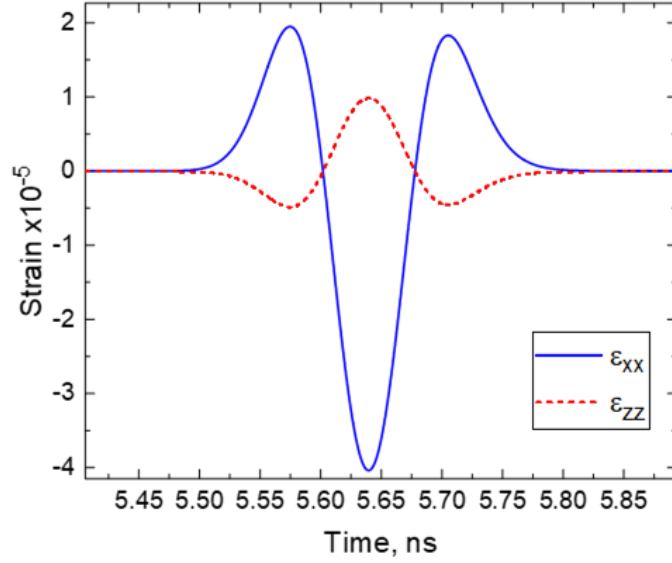

FIG. 8S. **Calculated Rayleigh SAW strain components.**  $\varepsilon_{xx}$  is in-plane,  $\varepsilon_{zz}$  is out-of-plane.

## V. LASER-INDUCED STRAIN $\varepsilon$ CALCULATION DETAILS

In calculations of laser-induced strain,  $\varepsilon$ , we performed a summation over a distribution of nucleation sites with individual threshold  $J_{PT}^*$  values. Fig. 9S(a) shows distribution of fraction of nucleation sites with a certain  $J_{PT}^*$  used in calculations centered at  $J_m = (J_T + J_S)/2$  with dispersion  $\sigma = (J_S - J_T)/6$ . Such value of  $\sigma$  corresponds to less than 0.01 % nucleation sites with  $J_{PT}^* = J_T$  and  $J_{PT}^* = J_S$  ensuring that the majority of sites are within the considered range  $J_T < J_{PT}^* < J_S$ . The distribution is normalized so that its integral between  $J_T$  and  $J_S$  is equal to 1.

Since each nucleation site has its own threshold fluence  $J_{PT}^*$  it also has its own AFM-FM transition temperature  $T_{PT}^*$  and therefore its own temperature dependence of physical properties which change upon transition. Fig. 9S(a) and (b) show linear thermal expansion coefficient and specific heat, correspondingly, of a nucleation site with a certain  $T_{PT}^*$  marked with a vertical line. The double arrow indicates that this value changes between sites. The specific heat data was taken from [23] and linear thermal expansion coefficient data was taken from [22].

In order to calculate  $\varepsilon(J)$  we had to calculate  $T(J)$  for initial temperatures  $T_0=295$  K,

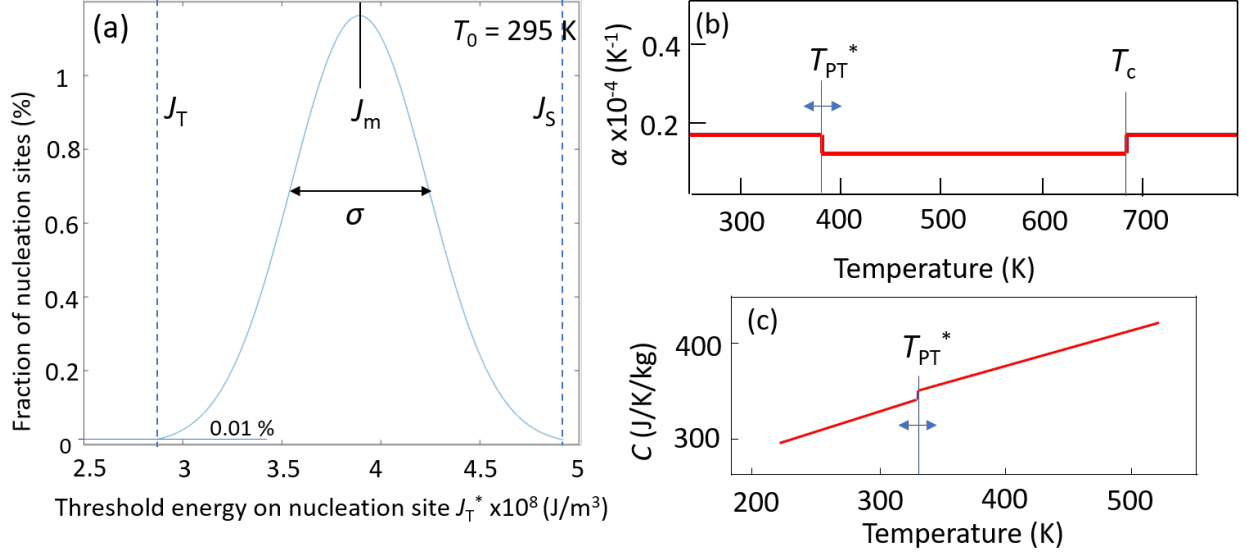

FIG. 9S. **Parameters used in calculations.** (a) The used distribution of nucleation sites with their local thresholds  $J_{PT}^*$ . (b) Approximation of linear thermal expansion coefficient  $\alpha$  adapted from [22]; (c) Approximation of specific heat  $C$  adapted from [23].

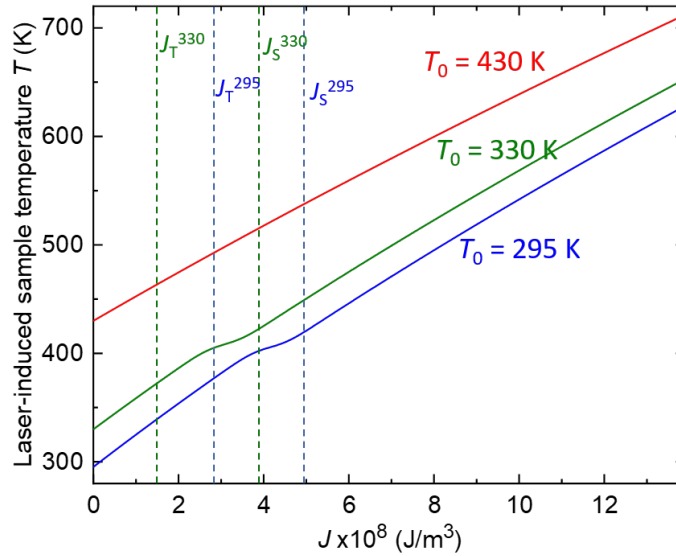

FIG. 10S. **Calculated laser-induced heating.** Calculated FeRh film temperature due to absorbed laser energy density  $J$  for three initial sample temperatures.

330 K and 430 K. The resulting graph is shown on Fig. 10S. The values of threshold and

saturation are shown as dashed vertical lines. For the largest used experimental  $J \approx 13 \text{ J/m}^3$  and for the largest  $T_0=430 \text{ K}$  the sample temperature rises up to  $700 \text{ K}$  which exceeds the Curie temperature  $T_c=680 \text{ K}$  [22]. We note that for larger laser energies (corresponding fluence is  $W_{max}=21 \text{ mJ/cm}^2$ ) we start damaging the FeRh film.

---

- [1] A. S. Komlev, D. Y. Karpenkov, D. A. Kiselev, T. S. Ilina, A. Chirkova, R. R. Gimaev, T. Usami, T. Taniyama, V. I. Zverev, and N. S. Perov, Ferromagnetic phase nucleation and its growth evolution in FeRh thin films, *Journal of Alloys and Compounds* **874**, 159924 (2021).
- [2] A. I. Zakharov, A. M. Kadomtseva, R. Z. Levitin, and E. G. Ponyatovskii, Magnetic and magnetoelastic properties of a metamagnetic iron–rhodium alloy, *Sov. Phys. JETP* **19**, 1348 (1964).
- [3] J. A. Arregi, O. c. v. Caha, and V. c. v. Uhlř, Evolution of strain across the magnetostructural phase transition in epitaxial FeRh films on different substrates, *Phys. Rev. B* **101**, 174413 (2020).
- [4] M. G. Loving, R. Barua, C. Le Graët, C. J. Kinane, D. Heiman, S. Langridge, C. H. Marrows, and L. H. Lewis, Strain-tuning of the magnetocaloric transition temperature in model FeRh films, *Journal of Physics D: Applied Physics* **51**, 024003 (2017).
- [5] A. Ceballos, Z. Chen, O. Schneider, C. Bordel, L.-W. Wang, and F. Hellman, Effect of strain and thickness on the transition temperature of epitaxial FeRh thin-films, *Applied Physics Letters* **111**, 172401 (2017).
- [6] Y. Xie, Q. Zhan, T. Shang, H. Yang, B. Wang, J. Tang, and R.-W. Li, Effect of epitaxial strain and lattice mismatch on magnetic and transport behaviors in metamagnetic FeRh thin films, *AIP Advances* **7**, 056314 (2017).
- [7] J. Cao, N. T. Nam, S. Inoue, H. Y. Y. Ko, N. N. Phuoc, and T. Suzuki, Magnetization behaviors for FeRh single crystal thin films, *Journal of Applied Physics* **103**, 07F501 (2008).
- [8] V. Saidl, M. Brajer, L. Horák, H. Reichlová, K. Výborný, M. Veis, T. Janda, F. Trojánek, M. Maryško, I. Fina, X. Marti, T. Jungwirth, and P. Němec, Investigation of magnetostructural phase transition in FeRh by reflectivity and transmittance measurements in visible and near-infrared spectral region, *New Journal of Physics* **18**, 083017 (2016).
- [9] C. Sánchez-Valdés, R. Gimaev, M. López-Cruz, J. Sánchez Llamazares, V. Zverev, A. Tishin,

- A. Carvalho, D. Aguiar, Y. Mudryk, and V. Pecharsky, The effect of cooling rate on magnetothermal properties of Fe<sub>49</sub>Rh<sub>51</sub>, *Journal of Magnetism and Magnetic Materials* **498**, 166130 (2020).
- [10] H. Kumar, D. R. Cornejo, S. L. Morelhao, S. Kycia, I. M. Montellano, N. R. Álvarez, G. Alejandro, and A. Butera, Strain effects on the magnetic order of epitaxial FeRh thin films, *Journal of Applied Physics* **124**, 085306 (2018).
- [11] C. Yu, H. Li, Y. Luo, L. Zhu, Z. Qian, and T. Zhou, Thickness-dependent magnetic order and phase-transition dynamics in epitaxial Fe-rich FeRh thin films, *Physics Letters A* **383**, 2424 (2019).
- [12] J. B. Staunton, R. Banerjee, M. d. S. Dias, A. Deak, and L. Szunyogh, Fluctuating local moments, itinerant electrons, and the magnetocaloric effect: Compositional hypersensitivity of FeRh, *Phys. Rev. B* **89**, 054427 (2014).
- [13] M. Arreguín-Hernández, C. Sánchez-Valdés, J. S. Llamazares, D. Ríos-Jara, V. Pecharsky, M. Blinov, V. Prudnikov, B. Kovalev, V. Zverev, and A. Tishin, Magnetoelastic transition and magnetocaloric effect in induction melted Fe<sub>100-x</sub>Rh<sub>x</sub> bulk alloys with  $x = 50, 51$ , *Journal of Alloys and Compounds* **871**, 159586 (2021).
- [14] F. Pressacco, V. Uhlir, M. Gatti, A. Bendounan, E. E. Fullerton, and F. Sirotti, Stable room-temperature ferromagnetic phase at the FeRh(100) surface, *Scientific Reports* **6**, 22383 (2016).
- [15] M. Mattern, J. Jarecki, J. A. Arregi, V. Uhlir, M. Rössle, and M. Bargheer, Speed limits of the laser-induced phase transition in FeRh, *APL Materials* **12**, 051124 (2024).
- [16] T. Saito, O. Matsuda, M. Tomoda, and O. B. Wright, Imaging gigahertz surface acoustic waves through the photoelastic effect, *J. Opt. Soc. Am. B* **27**, 2632 (2010).
- [17] Y. Sugawara, O. B. Wright, O. Matsuda, M. Takigahira, Y. Tanaka, S. Tamura, and V. E. Gusev, Watching ripples on crystals, *Phys. Rev. Lett.* **88**, 185504 (2002).
- [18] G. Farnell and E. Adler, 2 - elastic wave propagation in thin layers, in *Physical Acoustics*, Vol. 9, edited by W. P. Mason and R. Thurston (Academic Press, 1972) pp. 35–127.
- [19] D. W. Cooke, F. Hellman, C. Baldasseroni, C. Bordel, S. Moyerman, and E. E. Fullerton, Thermodynamic measurements of Fe-Rh alloys, *Phys. Rev. Lett.* **109**, 255901 (2012).
- [20] I. Viktorov, *Rayleigh and Lamb Waves: Physical Theory and Applications*, Ultrasonic Technology (Springer US, 2013).
- [21] I. Viktorov, Study of Rayleigh wave excitation, *Akusticheskij Zhurnal* **7**, 295 (1961), [in Rus-

sian].

- [22] M. R. Ibarra and P. A. Algarabel, Giant volume magnetostriction in the FeRh alloy, Phys. Rev. B **50**, 4196 (1994).
- [23] M. Richardson, D. Melville, and J. Ricodeau, Specific heat measurements on an Fe Rh alloy, Physics Letters A **46**, 153 (1973).
